# Supplementary material for: Boosting Unsupervised Segmentation Learning
Source: arXiv:2404.03392 source file (2024-11-28)
Supplement: Supplementary file 1 [file appendix2.tex]

% \subsection{Limitations}
% Our method exhibits challenges in scenarios where saliency within an image is unambiguous or when multiple objects are present in the scene. 
% Some visual examples can be seen in Fig. \ref{fig:main_fail}, where our method tends to segment all objects in the scene, whereas human annotators are inclined to select smaller and easily movable objects. Moreover, in instances where the salient object and the background share visual similarities our method encounters difficulty, making it challenging to distinguish between them accurately. 
% % This issue is particularly pronounced when the visual features of the salient and background objects closely resemble each other. The struggle to discern between these visually similar elements contributes to inaccuracies in segmentation, as depicted in various scenarios. 
% \begin{figure}[t]
%   \centering
%   \includegraphics[width=\linewidth]{figures/main_fail.pdf}
%   \caption{Some of the failure cases of our method from DUTS-TE \cite{wang2017learning}. In most cases the saliency is unambiguous or the background and the foreground are almost indistinguishable.}
%   \label{fig:main_fail}
% \end{figure}
